# Supplementary material for: Practical Bounds on Optimal Caching with Variable Object Sizes
Source: arXiv:1711.03709 source file (2018-07-05)
Supplement: Supplementary file 1 [file appendix.tex]

\section{Adversarial constant-factor bound}
